# Supplementary material for: Machine learning-based malware detection for IoT devices using control-flow data
Source: arXiv:2311.11605 source file (2023-11-20)
Supplement: Supplementary file 1 [file appendices.tex]

%----------------------------------------------------------------------------
\appendix
%----------------------------------------------------------------------------
\chapter*{\fuggelek}\addcontentsline{toc}{chapter}{\fuggelek}
\setcounter{chapter}{\appendixnumber}
\numberwithin{equation}{section}
\numberwithin{figure}{section}
\numberwithin{lstlisting}{section}
%\numberwithin{tabular}{section}
